# Supplementary material for: Embracing Safe Contacts with Contact-aware Planning and Control
Source: arXiv:2308.04323 source file (2023-08-08)
Supplement: Supplementary file 1 [file 80_appendix.tex]

\section*{APPENDIX}
%\section{APPENDIX}

\subsection{BiTRRT for contact-aware planning}

\begin{algorithm}[!ht]
\caption{BiTRRT for contact-aware planning}
\label{algorithm::BiTRRT_contact}
\begin{algorithmic}[1]
\State{\textbf{Input}: the goal mode $\sigma$, the root $\bm q_s^{init}$ and the goal $\bm q_s^{goal}$}
\State{\textbf{Output}: The tree $T$}
\State $T_1 \gets$ \texttt{initTree}($\bm q_s^{init}$),  $T_2 \gets$ \texttt{initTree}($\bm q_s^{goal}$)
\While{not \texttt{stopCondition}($T_1, T_2$)}
\State $\bm q_r^{rand} \gets$  \texttt{sampleRandomConfiguration}($C_{\mathcal{R}}$)
\label{lines::bitrrt_sample_start}
\State $\bm q_s^{rand} = \texttt{simplifiedEBmodel}(\bm q_r^{rand}, \sigma)$
\label{lines::bitrrt_sample_end}
\State $\bm q_{s1}^{near} \gets$ \texttt{NearestNeighbor}($T_1, \bm q_s^{rand}$)
\If{\texttt{refinementControl}($T_1, \bm q_{s1}^{near}, \bm q_s^{rand}$)}
\State $\bm q_{s1}^{new} \gets$ \texttt{extend}($\bm q_{s1}^{near}, \bm q_s^{rand}$)
\If{\texttt{transitionTest}($T_1, c(\bm q_{s1}^{near}), c(\bm q_s^{rand})$)  \\ \textcolor{white}{1} \hspace{6.5mm}  \textbf{and} $\bm q_{s1}^{new} \neq \text{null}$}
\State \texttt{addNewNodeAndEdge}($T_1, \bm q_{s1}^{near}, \bm q_s^{rand}$)
\State $\bm q_{s2}^{near} \gets$ \texttt{NearestNeighbor}($T_2,\bm q_{s1}^{new}$)
\If{\texttt{distance}$(\bm q_{s1}^{new}, \bm q_{s2}^{near}) < \epsilon$}
\State $T \gets$ \texttt{attemptLink}($T_1, \bm q_{s1}^{new}, T_2,\bm q_{s2}^{near}$)
\EndIf
\EndIf
\EndIf
\State \texttt{swap}($T_1, T_2$)
\EndWhile

\end{algorithmic}
\end{algorithm}

As shown in the algorithm \ref{algorithm::BiTRRT_contact}, the algorithm initializes two trees, one from the root configuration $\bm q_s^{init}$ and the other from the goal configuration $\bm q_s^{goal}$. It extends each tree in a loop until
 the trees are connected.
Lines \ref{lines::bitrrt_sample_start}-\ref{lines::bitrrt_sample_end} perform random sampling to generate a random configuration $\bm q_s^{rand}$ from $\mathcal{C}$.
Instead of sampling directly from $\mathcal{C}$, 
a random robot configuration $\bm q_r^{rand}$ is sampled first,
then the corresponding configuration of the elastic band $\bm q_b^{rand}$ is determined by the \texttt{simplifiedEBmodel} function defined in section \ref{section::simplified_model_of_eb}.
By stacking the $\bm q_r^{rand}$ and $\bm q_b^{rand}$ together, we obtain the sampled $\bm q_s^{rand}$.
Lines 7-13 expand one tree toward $\bm q_s^{rand}$ if the  \texttt{refinementControl} function allows it and the new node $\bm q_{s1}^{new}$ passes the \texttt{transitionTest}, which filters out irrelevant configurations that are not useful in finding low-cost paths \cite{2010TRRT}.
Lines 13-16 attempt to connect $\bm q_{s1}^{new}$ of the current tree to its nearest neighbor $\bm q_{s2}^{near}$ in the other tree.
Line 14 checks if these two nodes are physically feasible by checking the \texttt{distance} function. 
If feasible, the \texttt{attemptLink} function will merge the two trees.

\subsection{Force-regulating task}
\label{appendix::Force-regulating task}

In \cite{2021skin_nullspace}, a control method is proposed to make the robot arm reach the goal position in the cluttered environment while controlling the interaction forces applied to the environment. 
To keep the contact force small, the following control objective is proposed:
\begin{align*}
    L_f &= \frac{1}{2} \sum_{i=0}^{n_c} f_i^2 = \frac{1}{2} \bm f^T \bm f, 
      \bm f = [f_0, f_1, \dots, f_{n_c}]^T \\ 
     \nabla_t L_f &= \bm f^T \dot{\bm f}  = - \bm f^T \bm K_c \bm J_n \dot{\bm q} < 0 
\end{align*}
The joint velocity $\dot{\bm q}$ can be viewed as the control action, which can be selected as follows to make the  $\nabla_t L_f$ smaller than zero:

\begin{align}
\label{eq::nullspace_force_minimize}
    \dot{\bm q} = \gamma_f (\bm K_c \bm J_n)^T \bm f,
\end{align}
where the control gain $\gamma_f$ is a positive scalar.
However, keeping the force small can lead to oscillations: the control law defined in equation \ref{eq::nullspace_force_minimize} may keep the robot away from the contact object to minimize the contact force, while the objective of goal reaching will make the robot close to the object and re-establish contact again.

To keep the contact stable, instead of minimizing the contact force,
We can control the force's magnitude in the contact's direction. 
The corresponding objective is
\begin{align*}
     L_f &= \frac{1}{2} \sum_{i=0}^{n_c} (f_i -f_{d_i})^2 = \frac{1}{2} (\bm f - \bm f_d )^T (\bm f - \bm f_d ) \\
     \nabla_t L_f &= (\bm f - \bm f_d )^T \dot{\bm f }  = - (\bm f - \bm f_d )^T \bm K_c \bm J_n \dot{\bm q} < 0 
\end{align*}
The corresponding control task is then given by
\begin{align*}
    \dot{\bm q} = \gamma_f (\bm K_c \bm J_n)^T (\bm f - \bm f_d), \bm f_d \in [\bm 0, \bm f_{max}]
\end{align*}

\subsection{Derivation}

\subsubsection{Quasi-static model of soft contact}
\label{append::quasi_static_soft_contact}

\begin{equation}
 \mathop{\min}_{\bm q^{l+1}} \frac{1}{2} \| \bm q_{cmd}^{l+1} - \bm q^{l+1} \|^2_{\bm K_q}
 + \frac{1}{2}  \| \bm n_C^T (\bm x(\bm q^{l+1}) - \bm x(\bm q^0) )\|^2_{\bm K_C}
\end{equation}
For the unconstrained quadratic optimization problem, the optimal solution can be found by letting the gradient be zero:
\begin{align}
    \nabla_{\bm q^{l+1}} L 
    % &= \bm K_q (\bm q_{cmd}^{l+1} - \bm q^{l+1} ) + (\bm n_C^T \frac{\partial \bm x(\bm q^{l+1})}{\partial \bm q^{l+1}})^T  \bm K_C \bm n_C^T (\bm x(\bm q^{l+1}) - \bm x(\bm q^0) ) \\
    &= \bm K_q (\bm q_{cmd}^{l+1} - \bm q^{l+1} ) + \\
    & (\bm J_u (\bm q^{l+1}))^T  \bm K_C \bm n_C^T (\bm x(\bm q^{l+1}) - \bm x(\bm q^0) ) = \bm 0 \label{eq::soft_1}
\end{align}
Assume that the change in the joint position, $\bm q^{l+1} - \bm q^{l}$, is small and $\bm J_u^T (\bm q^{l+1})$ can be approximated with $\bm J_u^T (\bm q^{l})$.

Takes difference between the Eq. \ref{eq::soft_1} at the time step $l$ and $l+1$, we can obtain
\begin{align}
\bm K_q (\bm q_{cmd}^{l+1} - \bm q_{cmd}^{l} +\bm q^{l} - \bm q^{l+1}) + &
\\(\bm J_u (\bm q^{l}))^T  \bm K_C \bm n_C^T ( \bm x(\bm q^{l+1})  -  &\bm x(\bm q^{l})) = \bm 0 
\end{align}

Put Eq. \ref{eq::spring_force_model} into the above one, we obtain
% \begin{equation}
% \bm K_q (\bm q_{cmd}^{l+1} - \bm q_{cmd}^{l} +\bm q^{l} - \bm q^{l+1}) + (\bm J_u (\bm q^{l}))^T (\bm f_c^{l+1} - \bm f_c^{l}) = \bm 0 
% \end{equation}
\begin{align}
\label{eq::soft_2}
\bm K_q (\bm q_{cmd}^{l+1} - \bm q^{l+1}) + (\bm J_u (\bm q^{l+1}))^T \bm f_c^{l+1} = \\
\bm K_q (\bm q_{cmd}^{l} - \bm q^{l}) + (\bm J_u (\bm q^{l}))^T \bm f_c^{l}
\end{align}

By setting $l=0$ in Eq. \ref{eq::soft_1} and assume $\bm f_c^{0} = \bm 0$, we can obtain that 
\begin{equation}
\bm K_q (\bm q_{cmd}^{1} - \bm q^{1}) + (\bm J_u (\bm q^{1}))^T \bm f_c^{1} = \bm 0
\end{equation}

By induction, the Eq. \ref{eq::soft_2} can be simplified as 
\begin{equation}
\bm K_q (\bm q_{cmd}^{l+1} - \bm q^{l+1}) + (\bm J_u (\bm q^{l+1}))^T \bm f_c^{l+1} =
\bm 0
\end{equation}

\subsection{Contact stiffness identification}
\label{append::stiffness_identification}
In this section, the update law for the recursive least squares method is given:\\
 \textbf{Initialization:} 
 $\hat{\bm \phi }(0) = \hat{\bm \phi }_0, \bm P(0) =\bm P_{\bm \phi } = \text{Var}[\bm \phi ]$ \\
        \textbf{Recursion:} 
        
        Observe: $\bar{\bm z}(k)$ 
        
        Update: 
            $\bm K(k) = \bm P(\text{k-1})\bm H^T(k)\Big(\bm H(k) \bm P(\text{k-1}) \bm H^T(k)+\bm R(k)\Big)^{-1}$
            
            $\hat{\bm \phi}(k) = \hat{\bm \phi}(\text{k-1}) +\bm K(k)\Big( \bar{\bm z}(k) -\bm H(k) \hat{\bm \phi}(\text{k-1}) \Big)$ 
            
            $\bm P(k) = \Big(\bm I -\bm K(k) \bm H(k) \Big) \bm P(\text{k-1}) \Big( \bm I - \bm K(k) \bm H(k) \Big)^T+ \bm K(k) \bm R(k) \bm K^T(k)$

% \subsection{Contact detection via pesudo..}

% \subsubsection{Problem of the link isolation method in \cite{popov2021realtime_detection} for robot links with non-convex geometry}

% \begin{center}
% \textcolor{gray}{This part is to be done. This part is to be done. To do} \\
% \textcolor{gray}{This part is to be done. This part is to be done. To do} \\
% \end{center}

\subsection{Extensions of the contact-aware control}

Due to the modeling errors, the measured force $\bm f_{c}^{l}$ can be greater than the pre-defined threshold value $ \lambda_{max}$.
In this situation, the formulated QP can be infeasible to solve. 
In such cases, we introduce a modification to the formulation by adding a force-minimizing objective term: 
\begin{align}
    L_f = \epsilon_f \|  \bm f_{c}^{l+1} \|^2, \text{ if } f_{c_i}^l > f_{max} (i=1,\dots, n_c),
\end{align}
and the force magnitude constraint is relaxed as 
$\bm f_{c}^{l+1} \leq \bm f_{max} , 
   \bm f_{max} = max(\bm f_{c}, f_{max} ).$
% \begin{align}
%  \bm f_{c}^{l+1} \leq \bm f_{max} , 
%    \bm f_{max} = max(\bm f_{c}, f_{max} ).
% \end{align}

\subsection{Details about the simplified elastic band model}
\label{append::heuristic_eb}
In this section, we detail the implementation of the A* algorithm for finding the optimal path connecting the start point and the end point of the elastic band. 
The heuristic cost for the vertices $\bm v in \mathcal{V}^{eb}$ includes two parts.
The first one is the distance to the end point of the elastic band and is defined as 
\begin{equation}
    h_d(\bm v) = \| \bm v - \bm b_1 \|.
\end{equation}

The second heuristic guides the deformation
direction of the path. 
For mode 1, we want the path to be found around the lower region of the link surface in the world frame. 
In other words, we want the path of the band to be stable and will not fall back to the state without deformation.
The heuristic is defined as 
\begin{align}
    \bm n_v^{band} = \bm n_v - \left(\bm n_v \cdot (\bm b_1 -\bm b_0) \right) (\bm b_1 \bm b_0) \\
    h_{\sigma}(\bm v) = \left\{ {\begin{array}{*{30}{c}}
    { 0, \angle ( \bm d_b,  \bm n_v^{band}) \leq 90^{\circ} } \\
    { 2, \angle ( \bm d_b,  \bm n_v^{band}) > 90^{\circ}} \\
	\end{array}} \right.
\end{align}
where we check the angle between the normal vector of the vertex $\bm v$ and the deformation direction of the band $\bm d_b$.
Note that $\bm d_b$ depends on the mode $\theta$.
For mode 2, the deformation direction is opposite to the deformation direction in mode 1.
